# Supplementary material for: PASS: Peer-Agreement based Sample Selection for training with Noisy Labels
Source: arXiv:2303.10802 source file (2024-04-30)
Supplement: Supplementary file 2 [file clean.tex]

0,epochs,FINE,SmallLoss,PASS
0,50,0.82704,0.66028,0.6923767999999999
1,51,0.69504,0.65618,0.6951144
2,52,0.70858,0.66386,0.6918812
3,53,0.70572,0.65832,0.6948076
4,54,0.69542,0.6461,0.6959875999999999
5,55,0.6859,0.64358,0.6898752
6,56,0.69064,0.64812,0.6905595999999999
7,57,0.67958,0.64162,0.6931791999999999
8,58,0.67728,0.64298,0.6945716
9,59,0.67264,0.64678,0.6962944
10,60,0.67086,0.64492,0.6962235999999999
11,61,0.67012,0.64104,0.693958
12,62,0.66898,0.65008,0.6951379999999999
13,63,0.6683,0.6421,0.6955627999999999
14,64,0.66254,0.64736,0.6961999999999999
15,65,0.66874,0.63972,0.6975452
16,66,0.66376,0.63784,0.6951144
17,67,0.6655,0.65054,0.6973328
18,68,0.6667,0.64544,0.6949963999999998
19,69,0.66344,0.64426,0.696554
20,70,0.65356,0.64936,0.6959167999999999
21,71,0.66516,0.64258,0.6979464
22,72,0.66778,0.64464,0.6984892
23,73,0.6661,0.64784,0.6992916
24,74,0.66184,0.64206,0.6965068
25,75,0.66104,0.64058,0.6968371999999999
26,76,0.65738,0.63962,0.6996928
27,77,0.64608,0.64666,0.6992444
28,78,0.65854,0.64868,0.7020292
29,79,0.65828,0.64454,0.6998816
30,80,0.65406,0.63854,0.6999759999999999
31,81,0.66012,0.63914,0.6967428
32,82,0.6564,0.63704,0.7049791999999999
33,83,0.65932,0.6425,0.7033744000000001
34,84,0.6505,0.63636,0.7033744000000001
35,85,0.65022,0.6385,0.7034216
36,86,0.6494,0.63664,0.7034216
37,87,0.64816,0.6472,0.7041532
38,88,0.6489,0.64506,0.7063008
39,89,0.65084,0.64662,0.7040351999999999
40,90,0.64932,0.64768,0.7028316
41,91,0.64962,0.64696,0.7060175999999999
42,92,0.64656,0.64476,0.7072448
43,93,0.6546,0.64608,0.7078819999999999
44,94,0.6473,0.6476,0.7069616
45,95,0.6596,0.64848,0.7077167999999999
46,96,0.64822,0.6468,0.7086372
47,97,0.65274,0.64106,0.7059232
48,98,0.65408,0.64258,0.7084955999999999
49,99,0.65286,0.64204,0.7060647999999999
50,100,0.64916,0.65176,0.70446
51,101,0.65506,0.64326,0.712602
52,102,0.6482,0.64578,0.7084484
53,103,0.64848,0.6579,0.7100296
54,104,0.6472,0.6455,0.71213
55,105,0.6548,0.64348,0.7111152
56,106,0.65796,0.64904,0.7096284
57,107,0.65548,0.65088,0.7082596
58,108,0.65176,0.64436,0.7113512
59,109,0.65316,0.6478,0.7119648
60,110,0.6494,0.6507,0.7112567999999999
61,111,0.65334,0.64578,0.7132628
62,112,0.64898,0.65474,0.7120591999999999
63,113,0.65718,0.65074,0.7129088
64,114,0.65412,0.6491,0.7139
65,115,0.65278,0.65066,0.7173692
66,116,0.65354,0.64978,0.7119411999999999
67,117,0.65324,0.64926,0.7173927999999999
68,118,0.65494,0.64952,0.7165431999999999
69,119,0.65242,0.64516,0.7170388
70,120,0.65608,0.65162,0.7111152
71,121,0.6524,0.64616,0.7164724
72,122,0.65242,0.662,0.716024
73,123,0.65384,0.6483,0.7162599999999999
74,124,0.65272,0.64996,0.7177232
75,125,0.65386,0.64904,0.7181951999999999
76,126,0.65648,0.6512,0.717204
77,127,0.6504,0.65302,0.717086
78,128,0.65934,0.64836,0.7172276
79,129,0.65414,0.65514,0.7189739999999999
80,130,0.65588,0.65412,0.7159531999999998
81,131,0.65866,0.653,0.719446
82,132,0.65412,0.6478,0.7163544
83,133,0.6548,0.64876,0.7175579999999999
84,134,0.65276,0.64468,0.720154
85,135,0.6568,0.64768,0.7198943999999999
86,136,0.6561,0.65194,0.7198708
87,137,0.64776,0.65766,0.71744
88,138,0.65108,0.65252,0.7204844
89,139,0.6565,0.66488,0.7200123999999999
90,140,0.65376,0.64614,0.7207439999999999
91,141,0.66368,0.65108,0.7198236
92,142,0.65888,0.66296,0.7194223999999999
93,143,0.6533,0.6532,0.7204844
94,144,0.65552,0.66574,0.7204135999999999
95,145,0.65414,0.6549,0.7229388
96,146,0.65178,0.6586,0.7229151999999999
97,147,0.6566,0.65458,0.7212632
98,148,0.66472,0.65842,0.7250392
99,149,0.65708,0.65612,0.7239535999999999
100,150,0.65814,0.66042,0.7216408
101,151,0.66582,0.66436,0.7272339999999999
102,152,0.6671,0.66262,0.7299244
103,153,0.66856,0.66576,0.730302
104,154,0.66818,0.66956,0.7318832
105,155,0.66914,0.66636,0.7314584
106,156,0.67176,0.67014,0.732426
107,157,0.6717,0.6698,0.7326147999999999
108,158,0.67062,0.67096,0.7336531999999999
109,159,0.67112,0.67236,0.7345028
110,160,0.67252,0.6717,0.73632
111,161,0.67354,0.67356,0.7351872
112,162,0.67484,0.67372,0.7365796
113,163,0.6743,0.67662,0.7365796
114,164,0.67476,0.67426,0.7371931999999999
115,165,0.67596,0.67548,0.737264
116,166,0.67598,0.67518,0.7383968
117,167,0.6773,0.6752,0.7370515999999999
118,168,0.67836,0.6762,0.7388688
119,169,0.67786,0.67746,0.7390576
120,170,0.67866,0.67736,0.7394352
121,171,0.67882,0.67754,0.7403084
122,172,0.6798,0.67904,0.740686
123,173,0.67856,0.6796,0.7409927999999999
124,174,0.67916,0.67904,0.7402612
125,175,0.68006,0.67966,0.739742
126,176,0.68134,0.68068,0.7429044
127,177,0.67996,0.68254,0.7412288
128,178,0.68256,0.68012,0.7412523999999999
129,179,0.68262,0.6807,0.7425976
130,180,0.6818,0.68104,0.7431403999999999
131,181,0.68116,0.68254,0.7438719999999999
132,182,0.68248,0.6822,0.7437539999999999
133,183,0.68372,0.68224,0.7434236
134,184,0.68356,0.68288,0.7443676
135,185,0.68292,0.68414,0.7444147999999999
136,186,0.68396,0.68296,0.7459015999999999
137,187,0.68422,0.68368,0.7454531999999999
138,188,0.68502,0.68374,0.7445327999999999
139,189,0.68542,0.68436,0.7464444
140,190,0.68602,0.68502,0.7461376
141,191,0.68498,0.68512,0.7461848
142,192,0.68584,0.68506,0.7468691999999999
143,193,0.68632,0.68648,0.7474356
144,194,0.68742,0.68524,0.7466567999999999
145,195,0.68642,0.68616,0.746822
146,196,0.68822,0.68612,0.7473648
147,197,0.68816,0.68596,0.748002
148,198,0.68702,0.68738,0.7485919999999999
149,199,0.68858,0.68812,0.750244
150,200,0.68714,0.6878,0.748474
151,201,0.6878,0.68808,0.7509992
152,202,0.68886,0.68888,0.749536
153,203,0.68876,0.68802,0.750598
154,204,0.68748,0.68894,0.750244
155,205,0.68904,0.6888,0.7509048
156,206,0.68978,0.68912,0.7512588
157,207,0.69038,0.68942,0.750126
158,208,0.69014,0.68912,0.7520376
159,209,0.68978,0.69028,0.7521319999999999
160,210,0.69106,0.69106,0.752486
161,211,0.69186,0.6903,0.7520376
162,212,0.69086,0.69044,0.7511407999999999
163,213,0.69064,0.69062,0.7533828
164,214,0.6906,0.6907,0.7534772
165,215,0.69334,0.69174,0.7539256
166,216,0.69176,0.69128,0.7546335999999999
167,217,0.69198,0.69138,0.7539963999999999
168,218,0.6918,0.6926,0.7546099999999999
169,219,0.6912,0.69178,0.7547752
170,220,0.6916,0.6922,0.7551292
171,221,0.69202,0.69292,0.7560731999999999
172,222,0.6914,0.69262,0.75579
173,223,0.69288,0.69306,0.7556012
174,224,0.69308,0.69328,0.7561912
175,225,0.69264,0.69232,0.7572296
176,226,0.69324,0.69416,0.7558372
177,227,0.69318,0.69424,0.7570408
178,228,0.69318,0.69332,0.7561675999999999
179,229,0.69296,0.69318,0.756498
180,230,0.69432,0.69364,0.756616
181,231,0.69406,0.6947,0.7566632
182,232,0.69416,0.69436,0.7574891999999999
183,233,0.6944,0.69458,0.7585275999999999
184,234,0.69466,0.69514,0.7580319999999999
185,235,0.69468,0.6948,0.7580319999999999
186,236,0.69462,0.69416,0.75874
187,237,0.69454,0.6943,0.7584803999999999
188,238,0.69638,0.69534,0.7596132
189,239,0.69534,0.69488,0.7587636
190,240,0.69596,0.69502,0.7598256
191,241,0.69482,0.69658,0.7603683999999999
192,242,0.69596,0.69704,0.7599671999999998
193,243,0.69574,0.6958,0.7589288
194,244,0.69678,0.69546,0.7600616
195,245,0.697,0.6961,0.759802
196,246,0.69734,0.69658,0.7597548
197,247,0.69682,0.6964,0.7606515999999999
198,248,0.69686,0.69538,0.7615719999999999
199,249,0.6973,0.69618,0.7626812
200,250,0.69658,0.6961,0.7610528
201,251,0.6983,0.6962,0.7613832
202,252,0.69756,0.69804,0.7608404
203,253,0.69842,0.69712,0.7617608
204,254,0.69806,0.69698,0.7633891999999999
205,255,0.69938,0.6964,0.7626103999999999
206,256,0.6982,0.69668,0.7624924
207,257,0.69872,0.69724,0.7624216
208,258,0.69818,0.69698,0.76346
209,259,0.6979,0.69718,0.7638376
210,260,0.69888,0.69708,0.7629644
211,261,0.69998,0.69814,0.7636252
212,262,0.69942,0.69792,0.762398
213,263,0.69978,0.69792,0.7643568
214,264,0.70018,0.6977,0.7639083999999999
215,265,0.70032,0.69894,0.76464
216,266,0.69966,0.69898,0.7638848
217,267,0.7005,0.6988,0.765584
218,268,0.7007,0.69844,0.765466
219,269,0.70112,0.69884,0.76464
220,270,0.70064,0.6992,0.7663156
221,271,0.7013,0.69978,0.7649703999999999
222,272,0.70044,0.69888,0.7656312
223,273,0.70102,0.69814,0.766056
224,274,0.70146,0.69876,0.766056
225,275,0.70104,0.69952,0.763342
226,276,0.7014,0.69976,0.7661032
227,277,0.70178,0.69976,0.7659852
228,278,0.70078,0.7002,0.7673776
229,279,0.70194,0.70028,0.767944
230,280,0.70108,0.7008,0.7671652
231,281,0.70192,0.69954,0.7679675999999999
232,282,0.70286,0.70066,0.7671887999999999
233,283,0.70252,0.70088,0.7678731999999999
234,284,0.70326,0.70148,0.7678259999999999
235,285,0.70282,0.70172,0.7672595999999999
236,286,0.7027,0.70072,0.7627283999999999
237,287,0.70326,0.7011,0.7680856
238,288,0.70254,0.7017,0.7686519999999999
239,289,0.70356,0.70172,0.7683452000000001
240,290,0.70252,0.70184,0.7683452000000001
241,291,0.70324,0.70168,0.7695487999999999
242,292,0.70316,0.7021,0.7695723999999999
243,293,0.70336,0.70146,0.770304
244,294,0.7031,0.70246,0.7688408
245,295,0.70328,0.70248,0.7687228
246,296,0.70356,0.70306,0.769124
247,297,0.70366,0.70248,0.7691711999999999
248,298,0.70396,0.70236,0.7701388
249,299,0.7045,0.7031,0.7685103999999999
250,300,0.7053,0.70346,0.7705636
