# Supplementary material for: PASS: Peer-Agreement based Sample Selection for training with Noisy Labels
Source: arXiv:2303.10802 source file (2024-04-30)
Supplement: Supplementary file 3 [file f1.tex]

epochs,FINE,PASS,SmallLoss
50,0.681930527,0.8995733544,0.847718029
51,0.8244583355,0.8982934991,0.8496482098
52,0.8795803188,0.9006404418,0.847367907
53,0.890388255,0.8970344955,0.8495599929
54,0.9067631008,0.890739692,0.8505180341
55,0.9046564159,0.8886146751,0.8459485705
56,0.9097544034,0.8915969238,0.8468808098
57,0.909370361,0.8874180004,0.8483483434
58,0.9073696685,0.888529619,0.8495855037
59,0.9071055635,0.8925179051,0.8506698162
60,0.9070929351,0.8897709274,0.8504922967
61,0.9062321123,0.8884176018,0.8488975575
62,0.9053223344,0.8942238372,0.8501760195
63,0.9058135694,0.889550477,0.850283182
64,0.9026334911,0.8919566059,0.8509229493
65,0.9056422373,0.8872713576,0.8514843845
66,0.9038605312,0.8869502281,0.8496482098
67,0.9045993346,0.8947001894,0.8513991784
68,0.9066828664,0.8923715181,0.8498846123
69,0.9042466432,0.8905838521,0.8512356194
70,0.8972357436,0.894616755,0.8505960475
71,0.905157981,0.8895425487,0.8518935988
72,0.9077377813,0.8900584071,0.8522103339
73,0.9039860845,0.890818341,0.8527725035
74,0.9024209834,0.8880719,0.8511385484
75,0.9030100622,0.8876843851,0.8512428448
76,0.899877062,0.8854948195,0.8531172327
77,0.8915282986,0.8916087872,0.8527394499
78,0.9011285547,0.893280453,0.8547501835
79,0.9004936169,0.8888509533,0.8533132155
80,0.8976151623,0.8862316919,0.8533154141
81,0.9019423599,0.886192655,0.8510487626
82,0.8996383421,0.8861401873,0.8569329684
83,0.9019044047,0.8904890053,0.8558159015
84,0.8956620793,0.8854226976,0.8558797303
85,0.8945688933,0.8872724884,0.8560402883
86,0.8950117569,0.8847573565,0.8557849645
87,0.8931213171,0.8925252312,0.8563582801
88,0.8946929011,0.8915761356,0.857723688
89,0.8962355361,0.8927098319,0.8564037838
90,0.8953281839,0.8918876562,0.8554375757
91,0.8956829793,0.8922785567,0.8573356857
92,0.8930916127,0.8908423059,0.8585062959
93,0.8988408798,0.8929883716,0.8587566991
94,0.8932807277,0.8922659631,0.8581822991
95,0.9018644059,0.8946994503,0.8588335275
96,0.8947397687,0.8925332278,0.859534864
97,0.8973038148,0.8890001634,0.8576528508
98,0.8992638262,0.8896055168,0.8592455137
99,0.8973949844,0.890575982,0.8574960236
100,0.8954578162,0.8943123674,0.8568271051
101,0.8988753695,0.8902551762,0.8626556258
102,0.8944097181,0.8923805137,0.8592765948
103,0.8952533393,0.9007841812,0.860434254
104,0.8928896397,0.8916621966,0.8617566291
105,0.8994322658,0.8916218101,0.8609928539
106,0.9017580748,0.8955048791,0.8600931403
107,0.8998843088,0.8967191275,0.8590820712
108,0.8974390546,0.8918571489,0.8614106862
109,0.8983142615,0.8938019917,0.8620251798
110,0.8957669058,0.8970226006,0.8614092959
111,0.8982622834,0.8924434693,0.862791949
112,0.8946281902,0.8998396693,0.8617715449
113,0.9007298541,0.8969901133,0.8626756806
114,0.899105505,0.8962435297,0.8632941717
115,0.8970200969,0.897118057,0.8656118742
116,0.8982255088,0.8955661341,0.8620089078
117,0.8975579422,0.8956098667,0.8654369936
118,0.8992869517,0.8953677672,0.8647910176
119,0.8975006169,0.8925976008,0.8650670972
120,0.9004638937,0.8975970251,0.8614390926
121,0.8979885655,0.8908485194,0.8648061468
122,0.8979408538,0.9044960296,0.8643075135
123,0.8988931669,0.8938069697,0.8649789642
124,0.8976028554,0.8960180214,0.8655996121
125,0.8986568602,0.8958197374,0.8661774119
126,0.9007034547,0.8965224957,0.865498699
127,0.8964036019,0.8982836331,0.8652904696
128,0.9027351909,0.8949224987,0.8655785626
129,0.8989320655,0.900331241,0.8666464464
130,0.900878411,0.8993698157,0.8647047752
131,0.9020346684,0.8991493367,0.8667780937
132,0.8996715843,0.8949352891,0.864916298
133,0.9001239306,0.8948504423,0.8656775041
134,0.8986396254,0.8921660175,0.8673889819
135,0.9008196141,0.8949065253,0.8673390325
136,0.9011705425,0.8979033418,0.8671955983
137,0.8948289614,0.9023614205,0.8652783273
138,0.8974881092,0.8981554341,0.8679328109
139,0.901032774,0.9069657175,0.8671650051
140,0.898706733,0.8934753391,0.867728011
141,0.905553933,0.8977527473,0.867036064
142,0.9030797176,0.9058430266,0.8667619667
143,0.8985463153,0.8984203002,0.8675508685
144,0.9004174338,0.9077959873,0.8675025473
145,0.8993093166,0.8997093753,0.8693506994
146,0.8981466533,0.9026302373,0.8694619029
147,0.9012340519,0.9004734258,0.8682094066
148,0.9068960498,0.9021177399,0.8706508912
149,0.9012823903,0.9003184602,0.8699771742
150,0.9026477953,0.9045652912,0.8684668004
151,0.9082819654,0.90758108,0.8723929504
152,0.9095497715,0.9063417688,0.8740205201
153,0.9103223175,0.9085637519,0.8743387967
154,0.9099770944,0.9112032497,0.8754042236
155,0.9108786475,0.9089484384,0.8748640945
156,0.9127582422,0.9115081975,0.8756424666
157,0.9126511733,0.9113186612,0.876087086
158,0.9117259417,0.9120533557,0.8765309688
159,0.9122844266,0.9133401782,0.876910942
160,0.9133203623,0.9129146417,0.8779388014
161,0.9140112333,0.9141640698,0.8773700612
162,0.9146570568,0.9140316432,0.8782395189
163,0.9143215336,0.9163556505,0.8783029735
164,0.9147859055,0.9146179276,0.8787770483
165,0.9157948362,0.9153917242,0.8788878648
166,0.9155591751,0.9152333943,0.8793913093
167,0.9165296299,0.9153107389,0.8788727116
168,0.9173076779,0.9159216089,0.8798333791
169,0.9167531602,0.9170354061,0.8800862816
170,0.9173400579,0.9166490829,0.8802748201
171,0.9174573611,0.9166561535,0.8806668401
172,0.917987761,0.9178190372,0.8808550543
173,0.9175794608,0.9181667264,0.8811862069
174,0.9177065461,0.9178190372,0.8808256226
175,0.9183030894,0.9182106606,0.8804160423
176,0.9193015396,0.9188944883,0.8827747547
177,0.9182924113,0.9199404984,0.8814701595
178,0.9198797721,0.9185473704,0.8812956614
179,0.9202358609,0.9188466105,0.8821905121
180,0.919762484,0.9190326705,0.882614564
181,0.9190450356,0.920127883,0.8831636887
182,0.9200088001,0.9198798294,0.8828952609
183,0.9210375036,0.9200339736,0.8826759038
184,0.9207960573,0.9205007602,0.8834291318
185,0.9205795639,0.9214810263,0.8834604376
186,0.9210248968,0.9206840347,0.8845090244
187,0.9210892816,0.9210212164,0.8838953465
188,0.9214215733,0.9208775624,0.8834753328
189,0.9220243561,0.9214537645,0.8848049289
190,0.9226473985,0.9219337746,0.8845385559
191,0.9220791842,0.9220064661,0.8845064583
192,0.9222670375,0.9215259378,0.8849592582
193,0.9226155086,0.922806881,0.8852070781
194,0.9232884782,0.9219688314,0.8850087874
195,0.9226256815,0.9225746461,0.8849913735
196,0.9238055649,0.92235842,0.8854135735
197,0.9238244897,0.9222422519,0.8856446002
198,0.9229985199,0.9235218935,0.8860974393
199,0.9241908365,0.9241202756,0.8873132563
200,0.9230855238,0.9238885621,0.8861461861
201,0.923563794,0.9239041816,0.8875573351
202,0.9242686839,0.9244207368,0.8868467218
203,0.9241963479,0.9238607381,0.8875463769
204,0.9232695862,0.924339432,0.8872499585
205,0.9243988644,0.924425231,0.8874952044
206,0.9248713848,0.9247813691,0.8880445656
207,0.9249931093,0.9248735083,0.8871722286
208,0.9251313975,0.9245942925,0.8882403148
209,0.9249960593,0.9254323563,0.8883656238
210,0.9257953034,0.9259951479,0.8889145993
211,0.9261850592,0.9253221339,0.8883668449
212,0.925526421,0.9254855183,0.8879669317
213,0.9256169677,0.9256777482,0.8893135954
214,0.925463453,0.9256731444,0.8892490333
215,0.9271880166,0.926485306,0.8896064376
216,0.9263622067,0.9262161008,0.8901970641
217,0.9262092229,0.9260389291,0.8897793747
218,0.9263910259,0.9269176863,0.8900551075
219,0.9258962606,0.9262649075,0.8902265945
220,0.925997707,0.9267543244,0.8903320032
221,0.9263003204,0.927147942,0.8910763447
222,0.9259781453,0.9269943702,0.8910175313
223,0.9269194255,0.9273109315,0.8907042628
224,0.9270633011,0.9273445857,0.8913432375
225,0.9269335778,0.926653842,0.8917690854
226,0.9271161073,0.927976987,0.8908587117
227,0.9273843419,0.928034441,0.8918353959
228,0.9271352245,0.9273733474,0.8911380939
229,0.9271015358,0.927334952,0.8913541621
230,0.9281412518,0.927416602,0.8915577659
231,0.9277054794,0.9281779442,0.8913357289
232,0.9279640846,0.9282451362,0.8920018619
233,0.9281364279,0.928278552,0.8927427975
234,0.9283230707,0.9286181304,0.892356234
235,0.9280884313,0.928311953,0.8925458788
236,0.9281698525,0.927976987,0.8930077386
237,0.9278634618,0.9279530192,0.8926488053
238,0.9294316911,0.9286370994,0.8932608759
239,0.9286241819,0.9283693601,0.8928967091
240,0.9291308405,0.9284075709,0.8936519765
241,0.928251149,0.9295255941,0.8938158124
242,0.9288819578,0.9295438541,0.8935546222
243,0.9288487275,0.9291535653,0.8928780273
244,0.929344833,0.9288476128,0.8936160898
245,0.9296266718,0.9291818355,0.8936366067
246,0.9299321053,0.9294633843,0.893605866
247,0.9294978531,0.9295833758,0.8941264629
248,0.9296508883,0.9288524926,0.8944723295
249,0.9298413007,0.9291147178,0.8953190961
250,0.929512675,0.9291196189,0.8945137998
251,0.9302452798,0.9291912549,0.8946022584
252,0.9303382438,0.9306320312,0.8941861101
253,0.9305174796,0.9299120587,0.8947845027
254,0.9303846423,0.929811891,0.8957784685
255,0.9314513648,0.9294589275,0.8953362906
256,0.9304224946,0.9295971826,0.8951965322
257,0.9309182183,0.9299979018,0.8951505638
258,0.9307191385,0.929749687,0.8958243847
259,0.9303946769,0.9298927809,0.8960060731
260,0.9309080938,0.9298212387,0.8956291933
261,0.9316926891,0.9307034788,0.8960577949
262,0.9314177262,0.9304840863,0.8951352401
263,0.9314879716,0.9304218957,0.8965319304
264,0.9318973675,0.9303268397,0.8961782367
265,0.9319349674,0.9310260215,0.8967784968
266,0.9315888785,0.9311167355,0.8959735406
267,0.9318767848,0.9309260911,0.8972632167
268,0.9322677601,0.9307312149,0.8972500045
269,0.9323803451,0.9310168124,0.8965890933
270,0.9321628938,0.931211557,0.8975469559
271,0.9325084341,0.9317495256,0.8967399013
272,0.9319583112,0.9309831965,0.8972937486
273,0.9324955663,0.9303925656,0.8976315782
274,0.9328086412,0.9308975361,0.8975053467
275,0.9322612849,0.9313776667,0.8957478555
276,0.9326417028,0.9314245176,0.8975358623
277,0.9327256365,0.9315488034,0.8975226842
278,0.9322004458,0.9319867038,0.8982960516
279,0.9327772998,0.9319815542,0.8985984853
280,0.9322897554,0.932165507,0.8982220164
281,0.9328872849,0.9315784037,0.8988660652
282,0.9334309791,0.9323143571,0.8984265701
283,0.9331274087,0.9324088512,0.8986789781
284,0.9338391037,0.9327736811,0.8987116187
285,0.9334025749,0.9328822539,0.8984091703
286,0.9335036334,0.9321085443,0.8954128842
287,0.9337770183,0.9324411843,0.8988159927
288,0.9333899902,0.9324333419,0.8991811984
289,0.9341140506,0.932944371,0.8987941779
290,0.9331894953,0.9329675801,0.8990464957
291,0.9336386672,0.9329780489,0.8995697564
292,0.933768131,0.9329040073,0.8996480107
293,0.9337238293,0.9324488974,0.9002449994
294,0.9337255429,0.9332840161,0.8993028798
295,0.9339153868,0.9331740453,0.8992268321
296,0.9340519648,0.9347721962,0.8993592106
297,0.9340608201,0.9344224229,0.8994526852
298,0.9343356475,0.9350887849,0.9000125944
299,0.9345942495,0.9356764187,0.8990268397
300,0.9350987316,0.9366215828,0.9004119813
