# Supplementary material for: PASS: Peer-Agreement based Sample Selection for training with Noisy Labels
Source: arXiv:2303.10802 source file (2024-04-30)
Supplement: Supplementary file 4 [file precision.tex]

epochs,FINE,SmallLoss,PASS
50,0.5621674264,0.9843160342,0.9954196038
51,0.8205334009,0.9875531982,0.995437582
52,0.8938009399,0.9814581573,0.995416334
53,0.9142170875,0.982329343,0.9956955673
54,0.9529481823,0.9875949055,0.9959624972
55,0.9606296714,0.9871943472,0.9954030511
56,0.963738492,0.9863507393,0.996323573
57,0.9767125,0.9877448534,0.9955551752
58,0.9760857065,0.987888208,0.9960844191
59,0.9815832537,0.9899506792,0.9958344876
60,0.9838855914,0.9874551583,0.9955745476
61,0.983307002,0.9904535456,0.9955601471
62,0.9831665768,0.9884851415,0.99647782
63,0.9849510223,0.9910609269,0.9960899828
64,0.9868713134,0.9880863322,0.9964831788
65,0.9840601052,0.9901965724,0.9957124069
66,0.9874646467,0.992313874,0.995437582
67,0.986475108,0.9887260866,0.9958406714
68,0.9886548035,0.9915782222,0.9960868055
69,0.9885995263,0.9899116652,0.9966148218
70,0.9892403169,0.990224128,0.9962218694
71,0.9879457427,0.9903580663,0.9959737948
72,0.9891269704,0.9883888051,0.9958475363
73,0.984562657,0.9852969854,0.9958522864
74,0.9874286201,0.9883425504,0.9964847239
75,0.9895906068,0.9897356893,0.9962268457
76,0.9888410732,0.9869976719,0.9959838141
77,0.9891167504,0.9884247647,0.9958520073
78,0.9895513955,0.9886940308,0.9959971406
79,0.9887410903,0.9862756969,0.9961140412
80,0.9892484768,0.9899408252,0.9959854342
81,0.9888870101,0.9890008687,0.9959668604
82,0.9897487695,0.9919456909,0.9962703026
83,0.9899089398,0.9922507604,0.9962618166
84,0.99059027,0.991578363,0.9963903749
85,0.988952315,0.9919639984,0.9966477897
86,0.9909255259,0.9899110287,0.9961335414
87,0.9891513951,0.9893710454,0.9962659396
88,0.9910357384,0.9906303905,0.996021278
89,0.9911791154,0.9905353493,0.9965222167
90,0.9916272196,0.987508122,0.9962589375
91,0.9918653871,0.9892499309,0.9956357399
92,0.9913563632,0.9896840519,0.9962822175
93,0.9907648892,0.9918220774,0.9959024677
94,0.9906614594,0.9883244974,0.996024986
95,0.9894530518,0.9916174575,0.9962846902
96,0.9920828312,0.9899509876,0.9964171112
97,0.9905059403,0.9915210422,0.9964033731
98,0.992269794,0.9904762632,0.9960335672
99,0.9905076731,0.993076087,0.9958919539
100,0.9920942283,0.9863103732,0.9967811535
101,0.990191479,0.9907224697,0.9971989112
102,0.9914954573,0.9911115313,0.9961608979
103,0.992673381,0.9897732025,0.996296759
104,0.9900732337,0.9901660953,0.996053751
105,0.9915806437,0.9929730099,0.9959210415
106,0.9915051833,0.9923284015,0.9961672636
107,0.9914732462,0.9919989789,0.9960322494
108,0.9921255822,0.9921548149,0.9964307448
109,0.9917926657,0.9909043656,0.9968150032
110,0.9923317,0.9928162578,0.9965574376
111,0.9914454939,0.9912292746,0.996567095
112,0.9908025696,0.9923948124,0.9961803107
113,0.9906852569,0.9926995745,0.9968192107
114,0.9919210142,0.9936211267,0.996696872
115,0.9899248721,0.9930501534,0.9965866961
116,0.9910989633,0.9913999664,0.9968148979
117,0.9902805988,0.9922136816,0.9962086292
118,0.9911178651,0.9913965458,0.9960779854
119,0.9913169127,0.9924005903,0.9959546376
120,0.9917129602,0.9925924346,0.9968112069
121,0.9922500022,0.987713105,0.9962037724
122,0.9921335017,0.9909833462,0.9958227168
123,0.9919175751,0.9902082599,0.9968340579
124,0.9910878549,0.9919877209,0.9960844149
125,0.9914522541,0.992915429,0.9965906119
126,0.9916020558,0.991185028,0.9965859119
127,0.9921092128,0.9919084679,0.9963331013
128,0.9914074649,0.9922029356,0.9967121597
129,0.991572202,0.9927483418,0.9964684883
130,0.9927556005,0.9923876445,0.9967063216
131,0.9910522573,0.9935421817,0.9960937641
132,0.9929693092,0.9930196288,0.996581873
133,0.9928601342,0.9915037819,0.9964615376
134,0.9929547375,0.9922768148,0.9963486808
135,0.9913744477,0.993136074,0.9965986389
136,0.9929904166,0.9927129396,0.9963472483
137,0.9929006416,0.9930078063,0.995830936
138,0.9931709078,0.9923690843,0.9969781927
139,0.9921821072,0.9915940651,0.9960968281
140,0.9916837331,0.9926478842,0.9962262085
141,0.9906613568,0.9936404342,0.9960958073
142,0.9926727245,0.99214392,0.9960936363
143,0.9920274752,0.9919106843,0.9962248525
144,0.9924028893,0.9919478054,0.9962244825
145,0.992270499,0.9919315573,0.9964878057
146,0.993412292,0.9922078365,0.9967379646
147,0.9924153152,0.9937908836,0.9964796676
148,0.991705519,0.9915121096,0.9962485027
149,0.9918413332,0.9913666117,0.9963677929
150,0.9928961778,0.9932678243,0.9964815049
151,0.9927486884,0.9934223769,0.9967572902
152,0.9933340949,0.9935203322,0.9963974252
153,0.992778248,0.9933215555,0.9965231259
154,0.9926600904,0.9930175616,0.9965306182
155,0.9930123534,0.9932130748,0.9960341517
156,0.9929259568,0.9927960583,0.9962862339
157,0.9928118279,0.9929062261,0.996904572
158,0.9925730088,0.9926912243,0.9964156867
159,0.9929192461,0.9931599044,0.9960505414
160,0.9929339092,0.9932667617,0.9956920876
161,0.9928313606,0.9930588143,0.9960542073
162,0.9922804932,0.9926078927,0.995938941
163,0.9923873187,0.9929773561,0.9960616445
164,0.9926183282,0.9929529042,0.9961875374
165,0.9928568892,0.9927398684,0.9963105374
166,0.9924061319,0.9928495487,0.9958265242
167,0.9924208487,0.9929626639,0.9965548844
168,0.9924326255,0.9927475573,0.9960738111
169,0.9920899747,0.9930985691,0.9963194669
170,0.9920992444,0.9925349084,0.9961990644
171,0.9921010958,0.9923120129,0.9958372676
172,0.9917764354,0.9924410782,0.9957174002
173,0.9926594416,0.9923351844,0.9959630555
174,0.992105027,0.9924410782,0.9962032937
175,0.9920034443,0.9923358572,0.9960784321
176,0.9921301404,0.9922353838,0.9965819573
177,0.9921142615,0.991698742,0.996208236
178,0.9915864868,0.9923410115,0.9958425526
179,0.9921448116,0.9921237395,0.9958500606
180,0.9923588502,0.9920158513,0.9959746871
181,0.9919045088,0.9920332944,0.9961001419
182,0.9919200728,0.9920293473,0.9957350102
183,0.992157376,0.9922530364,0.9957331207
184,0.9919327625,0.9922602554,0.9959813037
185,0.992371311,0.9923857619,0.9959815578
186,0.9918261502,0.9924842228,0.9961107229
187,0.9916067721,0.9921578709,0.9955023511
188,0.9911723165,0.9918245274,0.9958608141
189,0.9917324065,0.9920543565,0.9959924516
190,0.9920725089,0.992061967,0.9958696895
191,0.9923941242,0.9920631188,0.9957488603
192,0.9916264746,0.9912848999,0.9957527436
193,0.9916322946,0.9917460952,0.9955142405
194,0.9914242323,0.9918423155,0.9961146454
195,0.991522653,0.9917422695,0.995873463
196,0.9913236074,0.9914091282,0.9959973724
197,0.9914333956,0.9914071371,0.9956383799
198,0.991419271,0.9918675597,0.9957624875
199,0.9915490791,0.9919868766,0.9960126878
200,0.99142076,0.9919831706,0.9960032865
201,0.9914289402,0.9916545772,0.9955354557
202,0.9913316167,0.9915537602,0.9960089326
203,0.9913303662,0.991653854,0.9960145628
204,0.9913143282,0.991333667,0.9958922277
205,0.9913338666,0.9916632468,0.9955348963
206,0.9912328387,0.9918879704,0.9961383779
207,0.990689826,0.9916706979,0.9958915835
208,0.9912373823,0.9915566834,0.9955415999
209,0.9914533876,0.9915707836,0.9956622529
210,0.9912489723,0.9915802384,0.9962648039
211,0.9909293192,0.9913506317,0.9957818418
212,0.991026319,0.9914625405,0.996137773
213,0.9914639628,0.9915749075,0.99590929
214,0.9912431811,0.9914657339,0.9956699723
215,0.9908389169,0.9915884637,0.9957923721
216,0.991367724,0.9916929714,0.9960358134
217,0.9908210343,0.9912540562,0.9960324731
218,0.99136822,0.9912693624,0.9957961764
219,0.9912507333,0.991149161,0.9959168136
220,0.9909259321,0.9914841111,0.9956794149
221,0.9909314023,0.9912733682,0.9959238023
222,0.9911432554,0.9913794187,0.9961614637
223,0.9909425828,0.9913848567,0.9958016738
224,0.9909451789,0.9911681857,0.9962830554
225,0.9912688054,0.9911560193,0.9958106742
226,0.9908376044,0.9911793089,0.9958029806
227,0.9913852947,0.9911803187,0.9961677879
228,0.9909464764,0.9911686919,0.9959243097
229,0.9911630634,0.9912766203,0.9959260844
230,0.9912897955,0.9908439612,0.9961656424
231,0.990848356,0.9908578373,0.9956881461
232,0.9911782401,0.9914008835,0.9959313992
233,0.9911812692,0.9911846078,0.9960561046
234,0.9911845483,0.9910822858,0.9959343038
235,0.9907470602,0.9909685386,0.9962920568
236,0.9909651195,0.9911793089,0.9962955073
237,0.9905264013,0.9909620781,0.9959367001
238,0.9909878015,0.990866195,0.9957048382
239,0.9908650886,0.9909695714,0.9960573277
240,0.9909823991,0.990862018,0.9961817934
241,0.9908582984,0.9908823445,0.9958279143
242,0.9905455954,0.9903433491,0.9958257186
243,0.9907610612,0.9911999638,0.9958200249
244,0.9903386021,0.991086362,0.9958262355
245,0.9905596038,0.9908760999,0.9961816752
246,0.9906731357,0.9907732437,0.9961814386
247,0.9905571823,0.9912074963,0.9960670853
248,0.9907758087,0.9911946833,0.9955972343
249,0.990563637,0.9906588337,0.995840527
250,0.9908812401,0.9907669248,0.9963067342
251,0.9900332534,0.990768242,0.9960708534
252,0.9911119432,0.9910101797,0.995949266
253,0.9903611266,0.9908893596,0.9959541456
254,0.990573839,0.9908875419,0.9958443729
255,0.990808819,0.9909891502,0.9959586395
256,0.9904669047,0.9908836444,0.9958395003
257,0.9906914297,0.990890917,0.9958391151
258,0.9910108815,0.9907785028,0.995844757
259,0.9907894607,0.9907811301,0.9957285174
260,0.9904761148,0.9907798167,0.9960789726
261,0.990490976,0.9910114588,0.9960823558
262,0.9907006818,0.9908997324,0.9958389867
263,0.990379726,0.9907908382,0.9960860947
264,0.9906021808,0.9908968822,0.9959654859
265,0.9904955601,0.9905867641,0.9962057664
266,0.9907038497,0.9906959951,0.9956105212
267,0.9901727136,0.9905848914,0.9959742897
268,0.9906091066,0.9906888513,0.9960917498
269,0.9902896525,0.9906941441,0.9958511498
270,0.9904998704,0.9905902401,0.9956243997
271,0.9902921269,0.9908151495,0.9957348228
272,0.9903887264,0.9905859616,0.9959745372
273,0.9906133635,0.9904672454,0.9960947511
274,0.9906192105,0.9905843562,0.9958587951
275,0.9901802284,0.9904859189,0.9958441167
276,0.9904017878,0.9902720938,0.9958590495
277,0.9900823138,0.9904891591,0.995976392
278,0.9903933563,0.9907120945,0.9957481602
279,0.9899764056,0.9906046512,0.9956336481
280,0.9901807846,0.9902864264,0.9958647643
281,0.9901924501,0.9908120198,0.9961044439
282,0.9899894286,0.9907181504,0.9962183366
283,0.9898765728,0.9906126384,0.9958685654
284,0.990211002,0.9905123154,0.9959860096
285,0.9899888631,0.9904072951,0.9961008596
286,0.9903113293,0.9902853254,0.9959592629
287,0.9901030324,0.9903988723,0.9958697044
288,0.9903091386,0.9896497936,0.9958727386
289,0.9903230875,0.9905155376,0.9955183639
290,0.9899846197,0.9904089236,0.995988714
291,0.9898868599,0.9906232668,0.9955253501
292,0.99020962,0.9899798855,0.9956428574
293,0.9898885724,0.9899708112,0.995881563
294,0.9902087906,0.9902011208,0.995873749
295,0.9903192624,0.9899852656,0.9958731176
296,0.9902151458,0.990317427,0.9956403253
297,0.9901086172,0.9904175996,0.9957580438
298,0.9902206655,0.9899835672,0.9956460515
299,0.9900125598,0.9901019947,0.9957544078
300,0.9899161773,0.9895676514,0.9958829462
