# Supplementary material for: PASS: Peer-Agreement based Sample Selection for training with Noisy Labels
Source: arXiv:2303.10802 source file (2024-04-30)
Supplement: Supplementary file 5 [file clean.tex]

0,epochs,FINE,PASS,SmallLoss
0,50,0.83454,0.53659,0.63712
1,51,0.65982,0.538131,0.63012
2,52,0.65774,0.5360379999999999,0.64234
3,53,0.66592,0.538959,0.6265
4,54,0.66948,0.539396,0.63278
5,55,0.66684,0.5381079999999999,0.63008
6,56,0.6707,0.5396259999999999,0.6295
7,57,0.67228,0.5382229999999999,0.63032
8,58,0.6673,0.537326,0.62876
9,59,0.6616,0.541558,0.6295
10,60,0.67516,0.5396949999999999,0.62174
11,61,0.67078,0.53843,0.6248
12,62,0.6619,0.543697,0.6224
13,63,0.6694,0.5418799999999999,0.62122
14,64,0.6644,0.5388439999999999,0.6311
15,65,0.67022,0.541696,0.62692
16,66,0.64988,0.540408,0.6271
17,67,0.6621,0.541512,0.61612
18,68,0.65694,0.541604,0.62776
19,69,0.65914,0.5424779999999999,0.6177
20,70,0.65422,0.5418109999999999,0.62486
21,71,0.6584,0.54441,0.6236
22,72,0.64532,0.542018,0.61776
23,73,0.65758,0.543306,0.61572
24,74,0.6457,0.5444559999999999,0.61664
25,75,0.64806,0.5444559999999999,0.61732
26,76,0.6467,0.545445,0.619
27,77,0.64634,0.545445,0.62438
28,78,0.64194,0.545974,0.61562
29,79,0.64576,0.545974,0.62076
30,80,0.63418,0.5456289999999999,0.61418
31,81,0.6408,0.5477909999999999,0.61982
32,82,0.63274,0.547055,0.61392
33,83,0.6369,0.547538,0.61644
34,84,0.64078,0.548389,0.62216
35,85,0.63444,0.5471929999999999,0.61552
36,86,0.63812,0.548044,0.6199
37,87,0.63276,0.5476989999999999,0.61658
38,88,0.6347,0.5490559999999999,0.62132
39,89,0.62824,0.549079,0.61854
40,90,0.63796,0.548665,0.6164
41,91,0.63618,0.5487799999999999,0.62084
42,92,0.63066,0.548573,0.61788
43,93,0.6304,0.551195,0.61298
44,94,0.62986,0.547492,0.61984
45,95,0.63166,0.548642,0.61742
46,96,0.6257,0.55062,0.61666
47,97,0.62792,0.5499299999999999,0.61588
48,98,0.62174,0.5514709999999999,0.6119
49,99,0.62972,0.55085,0.61648
50,100,0.62126,0.550505,0.61616
51,101,0.62582,0.5510569999999999,0.61544
52,102,0.6237,0.552368,0.61178
53,103,0.62474,0.5521379999999999,0.61518
54,104,0.62304,0.552828,0.60994
55,105,0.62656,0.552345,0.61634
56,106,0.6203,0.5508959999999999,0.61724
57,107,0.62562,0.5516779999999999,0.60988
58,108,0.62456,0.5542079999999999,0.61082
59,109,0.62408,0.5535869999999999,0.61192
60,110,0.61882,0.551931,0.61418
61,111,0.62456,0.554484,0.61074
62,112,0.62412,0.55223,0.6192
63,113,0.6216,0.550666,0.6108
64,114,0.62046,0.5498609999999999,0.61854
65,115,0.62118,0.553771,0.60592
66,116,0.61474,0.552667,0.61134
67,117,0.61948,0.5558409999999999,0.61032
68,118,0.62108,0.552299,0.60456
69,119,0.62464,0.555634,0.61422
70,120,0.61838,0.553403,0.61608
71,121,0.62152,0.5557949999999999,0.61816
72,122,0.60438,0.556508,0.60884
73,123,0.61768,0.556784,0.6092
74,124,0.6098,0.556485,0.61168
75,125,0.6154,0.555864,0.60322
76,126,0.60458,0.5548289999999999,0.61292
77,127,0.61008,0.556117,0.61202
78,128,0.6163,0.5568069999999999,0.61416
79,129,0.60786,0.555565,0.60528
80,130,0.61624,0.556002,0.61104
81,131,0.60986,0.556715,0.61022
82,132,0.60792,0.557014,0.61322
83,133,0.61192,0.5569679999999999,0.60532
84,134,0.61518,0.559176,0.60728
85,135,0.61248,0.557589,0.59948
86,136,0.61042,0.560832,0.6083
87,137,0.61502,0.5584629999999999,0.59622
88,138,0.61196,0.5585319999999999,0.60444
89,139,0.60882,0.5584629999999999,0.59684
90,140,0.6097,0.558394,0.59592
91,141,0.61038,0.560326,0.60008
92,142,0.60512,0.559889,0.60716
93,143,0.6109,0.560487,0.60516
94,144,0.6108,0.5597279999999999,0.60508
95,145,0.60074,0.560211,0.59228
96,146,0.613,0.561407,0.601
97,147,0.60264,0.559705,0.5939
98,148,0.6069,0.5606939999999999,0.60126
99,149,0.60994,0.5595209999999999,0.5902
100,150,0.60812,0.561522,0.60266
101,151,0.61156,0.5628099999999999,0.60662
102,152,0.61284,0.563615,0.6079
103,153,0.61466,0.563684,0.61174
104,154,0.61736,0.56511,0.60986
105,155,0.61836,0.5655469999999999,0.61134
106,156,0.61414,0.5660069999999999,0.61348
107,157,0.61592,0.565731,0.6119
108,158,0.61526,0.5664669999999999,0.61358
109,159,0.61708,0.56718,0.61284
110,160,0.6158,0.566651,0.61232
111,161,0.61704,0.567686,0.61088
112,162,0.61874,0.5682839999999999,0.61308
113,163,0.6162,0.5687209999999999,0.61376
114,164,0.61776,0.568974,0.6148
115,165,0.61812,0.5692499999999999,0.61402
116,166,0.62046,0.5687899999999999,0.614
117,167,0.61794,0.568583,0.61474
118,168,0.6185,0.569457,0.61414
119,169,0.61692,0.571665,0.61252
120,170,0.61668,0.570032,0.61288
121,171,0.61708,0.569641,0.61296
122,172,0.61616,0.570561,0.6129
123,173,0.61708,0.5708599999999999,0.61228
124,174,0.6169,0.570676,0.61472
125,175,0.61808,0.57017,0.61468
126,176,0.61818,0.571688,0.61382
127,177,0.6195,0.571642,0.61408
128,178,0.61732,0.5720559999999999,0.61366
129,179,0.61902,0.5724469999999999,0.61464
130,180,0.61854,0.572079,0.61562
131,181,0.618,0.572746,0.61416
132,182,0.62016,0.572861,0.61292
133,183,0.61802,0.573206,0.61492
134,184,0.61926,0.572171,0.61304
135,185,0.61844,0.5729759999999999,0.61504
136,186,0.61744,0.5734819999999999,0.61348
137,187,0.61858,0.573827,0.61546
138,188,0.61822,0.573712,0.61518
139,189,0.61844,0.5734589999999999,0.61442
140,190,0.618,0.5734589999999999,0.61476
141,191,0.61926,0.5735279999999999,0.61572
142,192,0.61918,0.5751379999999999,0.61498
143,193,0.61914,0.5747239999999999,0.61386
144,194,0.61872,0.5753449999999999,0.61376
145,195,0.61938,0.5753449999999999,0.61374
146,196,0.62026,0.5753219999999999,0.6158
147,197,0.61938,0.5751149999999999,0.61414
148,198,0.6209,0.574885,0.61558
149,199,0.62002,0.57569,0.61508
150,200,0.6208,0.5759659999999999,0.61616
151,201,0.62036,0.577231,0.61588
152,202,0.61946,0.576449,0.6142
153,203,0.6193,0.5763799999999999,0.61452
154,204,0.61932,0.575897,0.61484
155,205,0.61984,0.5767479999999999,0.61362
156,206,0.62048,0.577668,0.61612
157,207,0.61998,0.5775069999999999,0.61438
158,208,0.62016,0.577231,0.61614
159,209,0.62038,0.5772539999999999,0.61564
160,210,0.62118,0.5781509999999999,0.61554
161,211,0.62014,0.5783349999999999,0.61556
162,212,0.6198,0.577438,0.61624
163,213,0.62074,0.577231,0.61618
164,214,0.6213,0.577852,0.61432
165,215,0.6213,0.578243,0.6151
166,216,0.62078,0.578243,0.61574
167,217,0.62064,0.578887,0.61584
168,218,0.62164,0.578887,0.6157
169,219,0.62078,0.579255,0.61744
170,220,0.62142,0.5793699999999999,0.61676
171,221,0.62108,0.579186,0.6167
172,222,0.6204,0.5794159999999999,0.61626
173,223,0.62078,0.5796,0.61604
174,224,0.62124,0.5794159999999999,0.61658
175,225,0.62186,0.580152,0.61718
176,226,0.62262,0.579508,0.61686
177,227,0.62142,0.5811179999999999,0.61772
178,228,0.62022,0.580773,0.61622
179,229,0.62126,0.5808189999999999,0.617
180,230,0.62146,0.580543,0.61724
181,231,0.62208,0.580152,0.61696
182,232,0.62284,0.581371,0.6153
183,233,0.62186,0.5811179999999999,0.61722
184,234,0.62196,0.581463,0.6173
185,235,0.622,0.580359,0.61696
186,236,0.622,0.581141,0.61806
187,237,0.6212,0.581187,0.61764
188,238,0.62292,0.581693,0.6177
189,239,0.6218,0.5813479999999999,0.61868
190,240,0.62178,0.5818309999999999,0.61788
191,241,0.62326,0.5819689999999998,0.61764
192,242,0.62214,0.5815779999999999,0.618
193,243,0.6228,0.582291,0.61782
194,244,0.62246,0.5822679999999999,0.61706
195,245,0.6239,0.5820609999999999,0.6185
196,246,0.62178,0.5826359999999999,0.61806
197,247,0.62282,0.582452,0.61792
198,248,0.62226,0.581992,0.61782
199,249,0.62328,0.582291,0.61692
200,250,0.62484,0.5831189999999999,0.61738
201,251,0.62404,0.582843,0.61826
202,252,0.62436,0.58305,0.61848
203,253,0.6237,0.5828889999999999,0.61776
204,254,0.62366,0.583648,0.61914
205,255,0.62294,0.583579,0.61776
206,256,0.62326,0.584062,0.61812
207,257,0.62316,0.583464,0.61926
208,258,0.62408,0.584453,0.61864
209,259,0.62498,0.583832,0.61832
210,260,0.62474,0.584361,0.61966
211,261,0.62244,0.5842689999999999,0.62066
212,262,0.62464,0.5854189999999999,0.61932
213,263,0.624,0.584683,0.61972
214,264,0.62364,0.5848439999999999,0.6204
215,265,0.62256,0.5844299999999999,0.61978
216,266,0.62252,0.584867,0.62002
217,267,0.624,0.5842229999999999,0.61926
218,268,0.6242,0.58466,0.6203
219,269,0.62432,0.58489,0.61982
220,270,0.62358,0.585235,0.62038
221,271,0.62388,0.585741,0.62036
222,272,0.62428,0.5864309999999999,0.61942
223,273,0.62378,0.5858559999999999,0.61926
224,274,0.6242,0.585718,0.62114
225,275,0.62578,0.5861779999999999,0.62068
226,276,0.62454,0.585994,0.6206
227,277,0.62578,0.5861779999999999,0.61942
228,278,0.62462,0.5854649999999999,0.61886
229,279,0.62484,0.5864539999999999,0.62092
230,280,0.62542,0.5857870000000001,0.62098
231,281,0.62606,0.586661,0.62032
232,282,0.62568,0.586868,0.62098
233,283,0.62652,0.586776,0.62138
234,284,0.62504,0.5861779999999999,0.62044
235,285,0.6255,0.5864769999999999,0.62134
236,286,0.6256,0.587305,0.621
237,287,0.62484,0.5868909999999999,0.6212
238,288,0.6246,0.587397,0.62276
239,289,0.62536,0.587673,0.62122
240,290,0.62632,0.5877189999999999,0.62172
241,291,0.6264,0.587696,0.62108
242,292,0.62552,0.588064,0.62154
243,293,0.6263,0.588156,0.6216
244,294,0.6256,0.58788,0.62172
245,295,0.62656,0.58834,0.62364
246,296,0.6271,0.5883629999999999,0.62198
247,297,0.62616,0.5886389999999999,0.62224
248,298,0.62666,0.589214,0.62122
249,299,0.62494,0.588271,0.62258
250,300,0.6263,0.588846,0.6225
