# Supplementary material for: PASS: Peer-Agreement based Sample Selection for training with Noisy Labels
Source: arXiv:2303.10802 source file (2024-04-30)
Supplement: Supplementary file 6 [file f1.tex]

epochs,FINE,PASS,SmallLoss
50,0.6652859047,0.8681156189,0.8220862827
51,0.7350587827,0.8696238493,0.8205202436
52,0.781206983,0.8678811882,0.8263787371
53,0.7902059068,0.870383718,0.8248921435
54,0.8043044945,0.870100836,0.8235606705
55,0.8031297992,0.8696483382,0.8237605565
56,0.8077703925,0.8708583934,0.8239450008
57,0.8110127927,0.8697995457,0.8239805872
58,0.8059240959,0.8688384753,0.8240582955
59,0.8120927197,0.8725801947,0.8263223887
60,0.8064915565,0.8706482453,0.8281770849
61,0.811301944,0.8697159659,0.826776563
62,0.8086891182,0.8746213785,0.8248685441
63,0.8109763955,0.87310173,0.8274309619
64,0.8105670851,0.8701870643,0.8255617039
65,0.8118504646,0.872797236,0.8303532913
66,0.8116277891,0.8714377764,0.825935419
67,0.8130501513,0.8725836899,0.8301272902
68,0.8174811165,0.8728952712,0.8263899301
69,0.8154664247,0.8732379276,0.8289102589
70,0.813201601,0.8736759231,0.8268317552
71,0.8119902122,0.8758151641,0.8277224899
72,0.8157571845,0.8736372143,0.8284687775
73,0.8135178566,0.8747200616,0.8281095404
74,0.8118866388,0.875811526,0.828196694
75,0.8165777257,0.8755389087,0.8273733749
76,0.818008095,0.876891177,0.8277058981
77,0.8136139801,0.876891177,0.82741481
78,0.8122344835,0.8765084186,0.8284764284
79,0.8144547974,0.8769622938,0.8279968783
80,0.8000821512,0.8763770262,0.8245723598
81,0.8127887855,0.878561885,0.8314027935
82,0.8167458405,0.8776693517,0.8267829934
83,0.8149152005,0.8782424333,0.8305383871
84,0.8149624502,0.8791475418,0.8325258909
85,0.8171823297,0.8780210306,0.8286901866
86,0.8183069501,0.8787452187,0.8315147151
87,0.8227695372,0.8786600874,0.8259227863
88,0.8193676252,0.8800214357,0.8274851533
89,0.819899971,0.8797703372,0.8281968542
90,0.8184594281,0.879668656,0.8238066503
91,0.8160474399,0.8794552316,0.8326475236
92,0.8160332149,0.8795856167,0.8264402859
93,0.8119285262,0.8814949598,0.826829272
94,0.816987174,0.8783368717,0.8290924901
95,0.8184550877,0.8792400336,0.833014662
96,0.8182738348,0.8815661394,0.835534625
97,0.817946664,0.8806733454,0.8341239115
98,0.8172165642,0.8819240132,0.8303208921
99,0.8118628809,0.8813204273,0.8309201875
100,0.8199193096,0.8807836838,0.8361486258
101,0.8203115391,0.8813256184,0.8380602074
102,0.8191089605,0.8826390845,0.8379563014
103,0.8209030594,0.882703965,0.8346294002
104,0.8217569293,0.8831421326,0.8319271145
105,0.8225434793,0.8823923963,0.8353546586
106,0.8225253358,0.8812713014,0.8364528706
107,0.8230393757,0.8821552321,0.8395608675
108,0.8242973246,0.8845136671,0.8372607194
109,0.8213914867,0.883912656,0.8352695525
110,0.8243525383,0.8826538277,0.8379373917
111,0.8264589458,0.8847153693,0.8393896429
112,0.8234746537,0.8830126449,0.8341576008
113,0.8229305153,0.8812454042,0.8383240926
114,0.8250327386,0.8804753359,0.8349663917
115,0.8243667341,0.884393657,0.8366978563
116,0.8302852153,0.883178573,0.8296076826
117,0.8214226664,0.8860628948,0.8416711834
118,0.8252253317,0.8830293325,0.8358961791
119,0.8203565823,0.8858781753,0.8363958366
120,0.8268061452,0.8838382268,0.8353835547
121,0.8215649934,0.8858864907,0.8376447457
122,0.8322523512,0.8862968994,0.836390758
123,0.8273038545,0.8869487146,0.8377309737
124,0.8314676614,0.8867724968,0.8368216287
125,0.828328314,0.8860382963,0.8396655299
126,0.8328273433,0.885068944,0.8404377156
127,0.8278743349,0.8861737585,0.8398386053
128,0.8354123011,0.8870142982,0.8364558751
129,0.834453075,0.8856360839,0.8408817535
130,0.8283411374,0.8859358441,0.8384302992
131,0.8333758233,0.8867068629,0.8396820922
132,0.8330775317,0.8869281391,0.8384769873
133,0.8298187158,0.8868871675,0.8419305651
134,0.8290440404,0.8891205675,0.8444475199
135,0.8333791274,0.8873498945,0.8473644341
136,0.8305024615,0.8904532366,0.8430989471
137,0.8288573227,0.8883072913,0.8482175012
138,0.8317415833,0.8887740251,0.8395168922
139,0.8332969237,0.8882172016,0.8472218545
140,0.8348105563,0.8886964971,0.851524088
141,0.8326243373,0.8900501635,0.8483540325
142,0.8374079598,0.8894828911,0.840955835
143,0.8357310684,0.8902827499,0.8505553219
144,0.8319736282,0.8892501187,0.843342996
145,0.8383442669,0.8899482824,0.8454369029
146,0.8348235599,0.8910518983,0.8466224503
147,0.8364165943,0.8894997835,0.8475472907
148,0.8353019763,0.8904210432,0.8435772719
149,0.8341451394,0.8893816216,0.8517986399
150,0.8370951909,0.8909287747,0.8479681324
151,0.8377322505,0.8922013119,0.851589804
152,0.8364861719,0.8927764532,0.8500011588
153,0.8365122445,0.8930617699,0.8495290747
154,0.8371183728,0.8940475989,0.8500152363
155,0.83658097,0.8945213957,0.847106067
156,0.8374948094,0.8948805618,0.8481035567
157,0.8357914101,0.8946830321,0.8490941792
158,0.8365275799,0.895194637,0.8476922246
159,0.8369373635,0.8957750577,0.84891041
160,0.8371409468,0.8952664212,0.8495572378
161,0.8369773084,0.8961735617,0.8476912444
162,0.8375436942,0.8969208689,0.8484334238
163,0.8370100302,0.8971687314,0.8494054083
164,0.8385610636,0.897524135,0.8499320571
165,0.8374338999,0.8977205095,0.8499919996
166,0.8378587239,0.897094782,0.8506319094
167,0.8382659368,0.8972718987,0.8495290196
168,0.8385503114,0.8979460288,0.8505277314
169,0.8381725064,0.8998259003,0.850981572
170,0.8373369841,0.8983136876,0.8504584461
171,0.8384733675,0.8978382586,0.8505317606
172,0.8371268638,0.8988644348,0.8501666835
173,0.838281313,0.8989461931,0.8503348919
174,0.8373091406,0.8988752519,0.850323105
175,0.8380876486,0.898434071,0.8516024263
176,0.8380261035,0.899577847,0.8505445776
177,0.8373988408,0.8993144414,0.8502792242
178,0.8390781998,0.8999873431,0.8523355303
179,0.8378009429,0.900416606,0.8510239089
180,0.8378199931,0.9000073459,0.8504886174
181,0.8375153443,0.900497817,0.8508945149
182,0.8386556345,0.9005084364,0.852046148
183,0.8364215018,0.9009865936,0.8513960294
184,0.8368719393,0.8999980242,0.8526602648
185,0.8386102821,0.9010101075,0.8515057083
186,0.8377293602,0.9013154011,0.8526361458
187,0.8377417155,0.9015254344,0.8528955436
188,0.8386767524,0.9012918277,0.8520980318
189,0.8391474283,0.9009830528,0.85256532
190,0.8375537069,0.9009830528,0.8531083358
191,0.840091686,0.9009983134,0.8542553289
192,0.8393279812,0.9027504211,0.8532704714
193,0.8399432824,0.9021244581,0.852130859
194,0.8392126644,0.9024837878,0.853977993
195,0.839511449,0.9027066512,0.8529126702
196,0.8398965125,0.9026421745,0.8531283788
197,0.8395881348,0.9025521822,0.8538985122
198,0.8391806966,0.9022638913,0.85397281
199,0.8393317267,0.9029605265,0.8529357912
200,0.8405825569,0.9031991694,0.8526057148
201,0.8391453833,0.9042470997,0.8547883364
202,0.8395464797,0.9035720012,0.8524029894
203,0.8395914503,0.9036460323,0.8531990775
204,0.8408371858,0.9030504022,0.8543824245
205,0.8383621191,0.9040529103,0.8555963091
206,0.8389872938,0.9044904724,0.8533815322
207,0.8397548958,0.9042626098,0.8538463058
208,0.8398815247,0.9040245007,0.8540575438
209,0.8398148873,0.9041779022,0.8539113758
210,0.8389396236,0.9051292652,0.855253137
211,0.8399398389,0.9051097838,0.8544966911
212,0.8389767354,0.9042921181,0.8541486734
213,0.8402595008,0.904291622,0.8533201807
214,0.8392408447,0.9046936071,0.8550710457
215,0.8393939128,0.9049415525,0.8543096299
216,0.8402961205,0.9050305364,0.8540799852
217,0.8404360943,0.905629503,0.8546744488
218,0.8405852655,0.9055405523,0.8560187707
219,0.83945362,0.9058126979,0.8545451842
220,0.8390828833,0.905911604,0.85237972
221,0.8409919811,0.9059756839,0.8536394253
222,0.8410594143,0.9059511615,0.8537412882
223,0.8407174821,0.9064205634,0.8553987399
224,0.8411383274,0.9060400819,0.8551548854
225,0.8405185535,0.9067170137,0.8535354349
226,0.8406394043,0.9060747251,0.8552162614
227,0.8404988775,0.9074571921,0.8546839552
228,0.8409712948,0.9070279766,0.8556787933
229,0.8396251894,0.9072451352,0.8552662795
230,0.8408800167,0.9071415806,0.8557553747
231,0.8411788454,0.9065392526,0.8529871636
232,0.8409168326,0.9075853063,0.8555381598
233,0.840633352,0.9073239533,0.8557371873
234,0.8401126158,0.9077529806,0.8545724264
235,0.8413353664,0.9068058933,0.8536829559
236,0.8406848127,0.9076545771,0.8545294915
237,0.839991321,0.9074275396,0.8541474317
238,0.8413340105,0.9080388829,0.8545111748
239,0.8410377573,0.9078320406,0.8547454818
240,0.8412874238,0.9080683118,0.854945404
241,0.8400391669,0.9083196913,0.8559256384
242,0.8413867389,0.9077627393,0.8544749272
243,0.8414539077,0.9084622199,0.8547749054
244,0.8402255264,0.9083093855,0.8563655458
245,0.8418840689,0.9082653014,0.8547749874
246,0.8419382817,0.9086687197,0.8554182045
247,0.8411279906,0.9084668897,0.8545567148
248,0.8407694182,0.908206212,0.8561278831
249,0.841394974,0.908329076,0.8562769548
250,0.8412515374,0.9089931044,0.8563855654
251,0.8409039342,0.9088458009,0.8544023322
252,0.8405849169,0.9089341055,0.8541775768
253,0.8419309978,0.9090182425,0.8537157249
254,0.8412448721,0.9094895605,0.8541598856
255,0.8423466668,0.9093862674,0.8558413622
256,0.841338496,0.9098431155,0.8564777234
257,0.8420119133,0.9094654003,0.8545004179
258,0.8409022318,0.9099995374,0.8550952986
259,0.8422569961,0.9094250418,0.8553453441
260,0.8423438991,0.9100539944,0.8547478973
261,0.8411634009,0.9099754808,0.8543060367
262,0.8427111334,0.9109560896,0.856330487
263,0.8411347959,0.9105059691,0.8558826771
264,0.8419145033,0.9104660058,0.8549566244
265,0.8420764134,0.9102015172,0.8542011791
266,0.8404333157,0.9104856176,0.8554988874
267,0.842701305,0.9098918929,0.8536902373
268,0.8421193184,0.9103977183,0.8559070732
269,0.8441012253,0.9104609199,0.854623141
270,0.8421273554,0.9106221173,0.8556325053
271,0.8429742152,0.9112746307,0.8549203425
272,0.8424596444,0.9115962378,0.8536042189
273,0.841430755,0.9112839756,0.8555038777
274,0.8420429131,0.9111664723,0.8546642797
275,0.8413828644,0.9116023254,0.8542085929
276,0.8413216694,0.9113128975,0.8558319286
277,0.8418023602,0.9115137778,0.8559965074
278,0.8426547252,0.9109509838,0.8576904273
279,0.8424349623,0.9117928633,0.8560447766
280,0.8420469119,0.9113580838,0.8553283091
281,0.8412564743,0.911791869,0.855693799
282,0.8420164951,0.9121448917,0.855675147
283,0.8415987866,0.9119781689,0.8552669628
284,0.8417009038,0.9114695051,0.8551085561
285,0.8429592824,0.911768161,0.8553462848
286,0.8425159781,0.9122950223,0.8565798485
287,0.8421676861,0.9119874298,0.8549883011
288,0.8432859428,0.9125058937,0.8553999695
289,0.8427937448,0.9126518112,0.8558540277
290,0.8424842494,0.9126466383,0.8564608174
291,0.8420994865,0.9128040328,0.8555730644
292,0.8419471682,0.9128952593,0.8558741219
293,0.8429236752,0.9132828571,0.8555432675
294,0.8425541358,0.9128717664,0.8564608174
295,0.842893051,0.9131736364,0.8555035417
296,0.8418594416,0.9133699963,0.855425264
297,0.8424150253,0.913338788,0.8556990947
298,0.8428314231,0.9139586614,0.8551990369
299,0.8407321222,0.9132477509,0.855929721
300,0.8425041957,0.9136910628,0.8552031857
