# Supplementary material for: PASS: Peer-Agreement based Sample Selection for training with Noisy Labels
Source: arXiv:2303.10802 source file (2024-04-30)
Supplement: Supplementary file 7 [file precision.tex]

epochs,FINE,PASS,SmallLoss
50,0.5347406448,0.9916904396,0.7686705335
51,0.6645763341,0.9918422786,0.7715507375
52,0.7131291412,0.9920677621,0.7699259183
53,0.717910072,0.9918547769,0.7787139587
54,0.7305012377,0.9909030428,0.773087549
55,0.7307644092,0.9919059927,0.7750882735
56,0.7334026109,0.9916731859,0.7756740583
57,0.7358699361,0.9919717684,0.7751674339
58,0.7334012325,0.9917659388,0.7762905024
59,0.7430854624,0.9916391637,0.7782546361
60,0.7296101242,0.9912911079,0.7855510331
61,0.7370108589,0.991590729,0.7819207414
62,0.739358514,0.9917987593,0.7814742063
63,0.7374520042,0.9919621823,0.7850921812
64,0.7398757758,0.991725102,0.7763633167
65,0.7378944328,0.9917685482,0.784381275
66,0.7495513125,0.9914938707,0.779445335
67,0.7437947943,0.9917021059,0.7916244778
68,0.7514787726,0.9920217506,0.7794954171
69,0.7480576178,0.9913991797,0.789168975
70,0.7486005194,0.9928522178,0.7819401457
71,0.7448495574,0.9925694757,0.7837740285
72,0.7567228944,0.9925367661,0.7886406534
73,0.7469351364,0.9924274639,0.7896799459
74,0.7523753557,0.9925067586,0.7891275759
75,0.7559032177,0.9921267555,0.7877427537
76,0.7582612166,0.9927732434,0.7869344615
77,0.753815655,0.9927732434,0.7829042133
78,0.7550728403,0.9915803418,0.7901555612
79,0.7550661516,0.99221174,0.7860311502
80,0.7469448575,0.991827719,0.7868622877
81,0.7563765751,0.9921745623,0.7904271211
82,0.7657641845,0.9918489631,0.7894884463
83,0.7611174914,0.992045019,0.791851914
84,0.7587104859,0.9922459486,0.7900298396
85,0.7651330765,0.9921660329,0.7904622679
86,0.7639771928,0.9921152534,0.7904942663
87,0.7722537849,0.9924250837,0.7866636525
88,0.7673179539,0.9926321954,0.7850825232
89,0.7721315625,0.9922556673,0.7877953978
90,0.7642430422,0.9926269578,0.7844590738
91,0.7627931456,0.9921886281,0.7910828432
92,0.7663504443,0.9926257244,0.7863238536
93,0.7620875122,0.9920351085,0.7902074642
94,0.7679060155,0.9922332777,0.7878732643
95,0.7683130384,0.9920609836,0.7938915418
96,0.7720577489,0.9928410005,0.7972149144
97,0.7702250652,0.9924557362,0.7962112194
98,0.7735696846,0.9922891711,0.7948490503
99,0.7624588317,0.9922179051,0.7922450571
100,0.7768485728,0.9918999062,0.7982510483
101,0.7741937146,0.9919705573,0.8008842929
102,0.7743097281,0.9921768137,0.8034203583
103,0.7755637968,0.9925482905,0.7972707501
104,0.7776453999,0.9923080495,0.798050595
105,0.7761255018,0.9918644049,0.7972441756
106,0.7803578679,0.9920933798,0.7978165247
107,0.7772979042,0.9923545619,0.8066014977
108,0.7793864167,0.9925138246,0.8033469866
109,0.7765417623,0.9924431522,0.8003302265
110,0.7833837009,0.9927329718,0.8016567354
111,0.7817459966,0.992455346,0.8057779856
112,0.7787872721,0.9928618221,0.7938949148
113,0.7799100243,0.9923405475,0.8045463197
114,0.782995978,0.9922666525,0.7952523924
115,0.7817703644,0.9928816382,0.8063328287
116,0.7927872452,0.9925554053,0.7944605068
117,0.7797132014,0.9926598597,0.8086325737
118,0.7827797899,0.9928002556,0.8064483553
119,0.7750357943,0.9926571319,0.799917627
120,0.7863862321,0.9925652815,0.7974617753
121,0.7784708666,0.9924730971,0.7984782571
122,0.8025078362,0.9921729027,0.8038290461
123,0.7874229691,0.9927342084,0.8050599641
124,0.797650485,0.9928542834,0.8022306671
125,0.7901566153,0.9925981155,0.8116893883
126,0.8030034019,0.9925221825,0.8053498207
127,0.7934527731,0.9924774443,0.8053403568
128,0.7973458156,0.9927964555,0.8000274655
129,0.8023965769,0.9924079164,0.8115033963
130,0.7895776236,0.9922898281,0.8044888929
131,0.7997308441,0.9924855043,0.8064863916
132,0.8008170449,0.9924276159,0.8029514297
133,0.7942868252,0.9924269921,0.8126510761
134,0.7911028896,0.9928269003,0.8140025469
135,0.7978345587,0.9923117159,0.8232511112
136,0.7961275601,0.9926635216,0.8117279871
137,0.791010006,0.9925707202,0.8267734825
138,0.7963918038,0.9931274748,0.8106022678
139,0.8004023261,0.9924472135,0.8251525894
140,0.8014457898,0.9931875683,0.8307785667
141,0.798516107,0.9927184682,0.823906197
142,0.8077352625,0.9924664012,0.8101783584
143,0.8015949358,0.9928436381,0.8224767
144,0.7974878143,0.992341021,0.8144191462
145,0.8120929252,0.9927169771,0.8267262081
146,0.7990626227,0.9927938947,0.8212331789
147,0.8084830279,0.9927104091,0.8278467903
148,0.804053332,0.9927847534,0.8175912854
149,0.800529223,0.9927696639,0.8356895307
150,0.8051561045,0.9924882548,0.821475122
151,0.8033411421,0.9926892423,0.8225270441
152,0.8010246581,0.9925160796,0.8197689105
153,0.7997392895,0.9928229335,0.8163580886
154,0.798475937,0.9924748018,0.8183078597
155,0.7971707904,0.9926025641,0.8139474778
156,0.8012040287,0.9925476281,0.8134767103
157,0.7980367948,0.9926049641,0.8157529356
158,0.7993249576,0.9924319044,0.8129443826
159,0.7984755849,0.9923805937,0.8148500151
160,0.7996167586,0.9923126446,0.8159581106
161,0.7985483039,0.992326624,0.8149436839
162,0.7979637427,0.9926381038,0.8141401016
163,0.7991851068,0.9924618228,0.8147216688
164,0.7997853435,0.9926470096,0.8145414577
165,0.798283197,0.9925899782,0.8151837086
166,0.7970934833,0.9922808553,0.8159121622
167,0.7993306998,0.9927632899,0.8141366509
168,0.7992458839,0.9926532308,0.8156924427
169,0.7999560644,0.9926212041,0.817400813
170,0.7992033707,0.9924791157,0.8165487279
171,0.8001744202,0.9922923572,0.8165711936
172,0.7993430801,0.9926069621,0.8162080587
173,0.7999619519,0.9923691787,0.8168567666
174,0.7990152771,0.9924875815,0.8150361239
175,0.7990338973,0.9924809314,0.8164916351
176,0.7988946699,0.9922595682,0.8159479353
177,0.7972651331,0.9919573803,0.8154596641
178,0.8006717782,0.9923850916,0.8180654614
179,0.7980489201,0.9925107644,0.8158762326
180,0.7984108768,0.992385397,0.8145578874
181,0.7984585769,0.9922738295,0.8160867089
182,0.7981838319,0.9921549978,0.8182926332
183,0.7972361827,0.99240033,0.8160842789
184,0.7968539136,0.9922660853,0.8188895131
185,0.7993548521,0.992698241,0.8161179429
186,0.7990942972,0.9925242467,0.8185349913
187,0.7982960132,0.9924085334,0.8173567525
188,0.7995850439,0.9922267031,0.8166747191
189,0.7999482767,0.9921030337,0.8177579945
190,0.7985009587,0.9921030337,0.8181118361
191,0.8004071263,0.9920438676,0.8186801785
192,0.7996208148,0.9925457177,0.81812973
193,0.800328679,0.9921803609,0.8176884574
194,0.7998208353,0.9919490846,0.8198254925
195,0.7996811573,0.9922487084,0.8186504712
196,0.799481318,0.9921884674,0.8173651752
197,0.7997658079,0.9923055725,0.8194539121
198,0.7982393303,0.992182545,0.818468799
199,0.7990285422,0.9921934476,0.8176825103
200,0.7998551277,0.9921971787,0.816517667
201,0.798582228,0.9921545013,0.8191559654
202,0.7996629654,0.9921438864,0.817739956
203,0.7998263501,0.9923224161,0.8183909761
204,0.8011876899,0.9920765086,0.8194740043
205,0.7980867196,0.9924468835,0.8217385681
206,0.7983230578,0.9919813727,0.8174111152
207,0.7995236993,0.9918597568,0.8192172401
208,0.7995356965,0.9918558753,0.8181494025
209,0.7993062501,0.9920353602,0.8183559422
210,0.7977761314,0.992286231,0.8199260817
211,0.7996142051,0.9920502076,0.8190676751
212,0.7987929483,0.9919781874,0.8181771073
213,0.7995414637,0.9922142338,0.8172985457
214,0.7980232307,0.9920435805,0.820629399
215,0.7981918121,0.991929706,0.8191998916
216,0.7995535092,0.9920489461,0.8184699388
217,0.7998070058,0.9921173255,0.8190586074
218,0.7992639819,0.9919982126,0.8206614121
219,0.7986248768,0.9919437672,0.8177345276
220,0.7977646648,0.991945362,0.8158249372
221,0.8001081598,0.9922404454,0.8172709422
222,0.8006647257,0.9919459997,0.8177085685
223,0.8000180589,0.9923649598,0.8197180011
224,0.8001561804,0.9920649997,0.8190469998
225,0.7990352226,0.9921344679,0.8168022174
226,0.7986327398,0.9920067642,0.818908693
227,0.7993242338,0.9920288503,0.8176831114
228,0.8006953482,0.9918460534,0.8198969468
229,0.7984747842,0.992084116,0.8188611289
230,0.7997158772,0.9922585359,0.8192287227
231,0.7996070554,0.9918967683,0.8163538641
232,0.7987831705,0.9919137126,0.8204221317
233,0.7991616352,0.991850881,0.8192232213
234,0.7985177711,0.9920335671,0.8178678075
235,0.7998358991,0.9920184535,0.8171280803
236,0.7991195262,0.9922664812,0.8172617446
237,0.7989205075,0.9919111595,0.8171451245
238,0.7991858277,0.99215525,0.8175056236
239,0.7996493731,0.9922692277,0.8170474562
240,0.7999385112,0.9920385923,0.8178563687
241,0.79752306,0.9922182069,0.8191234733
242,0.7997936273,0.9919165829,0.8172450937
243,0.7994022258,0.9920448648,0.8177108116
244,0.798289949,0.9918669317,0.8200410692
245,0.7991019293,0.9920417298,0.8172120703
246,0.8006555613,0.9919312217,0.8182499788
247,0.7990295465,0.991869494,0.8173947384
248,0.7990293464,0.9920407888,0.8192159935
249,0.7989996827,0.9918672521,0.8200458192
250,0.7977488602,0.9918196527,0.8198271237
251,0.7979267291,0.9919340795,0.8169737535
252,0.7973524414,0.9918186873,0.816562862
253,0.7992939555,0.9921121529,0.8165770124
254,0.7985677708,0.9918861094,0.8160607479
255,0.8002860216,0.9918260831,0.8189413342
256,0.7989516299,0.9918918451,0.819384425
257,0.7997626903,0.9920608152,0.8163512046
258,0.7978968485,0.9916613418,0.8174654638
259,0.7987548345,0.9915934625,0.8179780469
260,0.7990182467,0.9918369915,0.8163339915
261,0.7993361454,0.9918357097,0.8151161519
262,0.7994916985,0.9918517037,0.8183397766
263,0.7982083877,0.9920773234,0.8175498277
264,0.799317973,0.9918437145,0.816026431
265,0.8002565631,0.991955923,0.8156398632
266,0.7984763568,0.9918440344,0.8169048208
267,0.7999300654,0.9917760661,0.8154518487
268,0.799149979,0.9919590789,0.8171535426
269,0.801244237,0.9917854187,0.8160788897
270,0.7995941906,0.9916135589,0.8167906302
271,0.8003144897,0.9919150235,0.8160153028
272,0.799467845,0.9915718423,0.8152397658
273,0.798687884,0.9917989261,0.8174654971
274,0.7990660193,0.9917969992,0.8151647948
275,0.7972372654,0.9918622254,0.8149936309
276,0.7980355914,0.9916832088,0.8168515759
277,0.7976973327,0.9917446142,0.8178955891
278,0.799443749,0.9917934641,0.8201889635
279,0.7990482374,0.9918072655,0.8168546668
280,0.7982167377,0.9919745071,0.8160167831
281,0.7969038167,0.9915751372,0.8169023477
282,0.7980019371,0.9918130291,0.8164012385
283,0.7969592291,0.9916942617,0.8156584118
284,0.7981023943,0.9916858121,0.8161658114
285,0.7991621606,0.9917488113,0.8157753122
286,0.7986057806,0.9915256663,0.8173897376
287,0.7987547231,0.9915784295,0.8154802644
288,0.8001513145,0.9917030181,0.8148070594
289,0.7990783358,0.9915896041,0.8164250823
290,0.7980689081,0.9915316187,0.8167343268
291,0.797591415,0.9917658786,0.816215405
292,0.7980374962,0.9914779674,0.8162149776
293,0.7985646793,0.9918895185,0.8158049326
294,0.798647652,0.9916511853,0.8167343268
295,0.7983499822,0.9915405318,0.8142873357
296,0.79684215,0.9917751874,0.8153989186
297,0.7981044496,0.9914277221,0.8155138742
298,0.7982128156,0.9916115382,0.8156992457
299,0.7971089446,0.9917153106,0.8155231999
300,0.798104706,0.9916648431,0.8147770987
